# Supplementary material for: Generative Semantic Manipulation with Contrasting GAN
Source: arXiv:1708.00315 source file (2017-08-01)

Horse -&gt; Zebra

Input

CycleGAN

Ours

Zebra -&gt; Horse

Input

CycleGAN

Ours

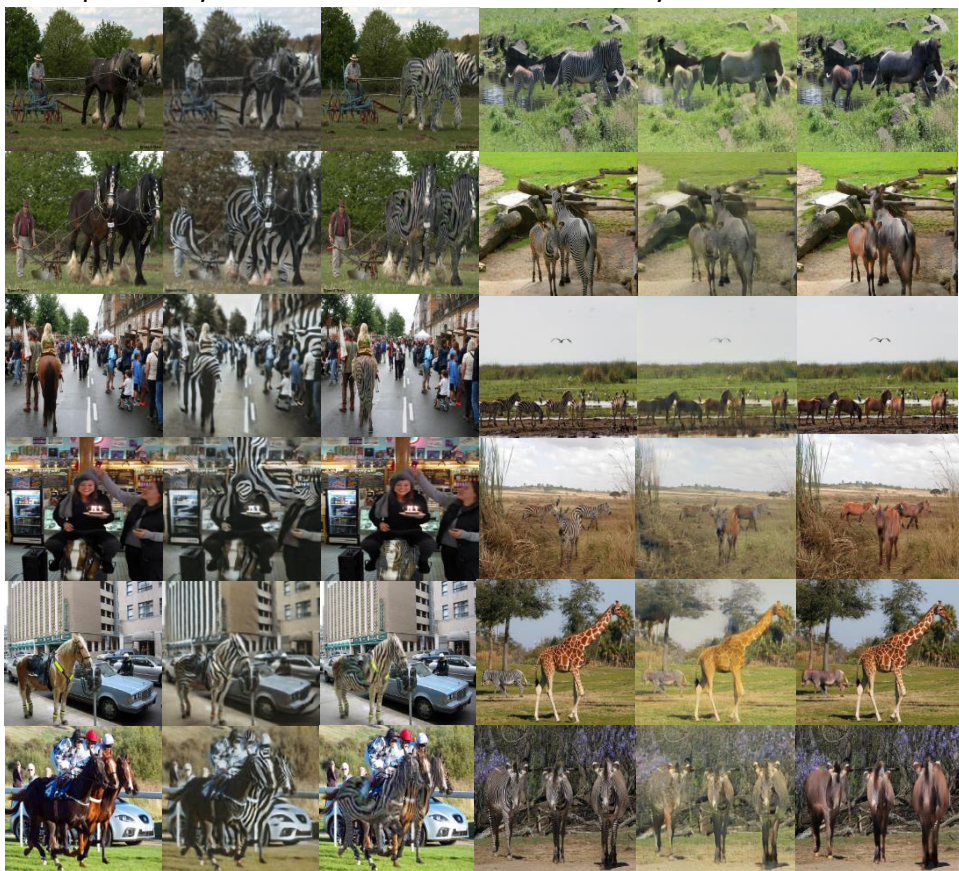

Horse -&gt; Zebra

Input

CycleGAN

Ours

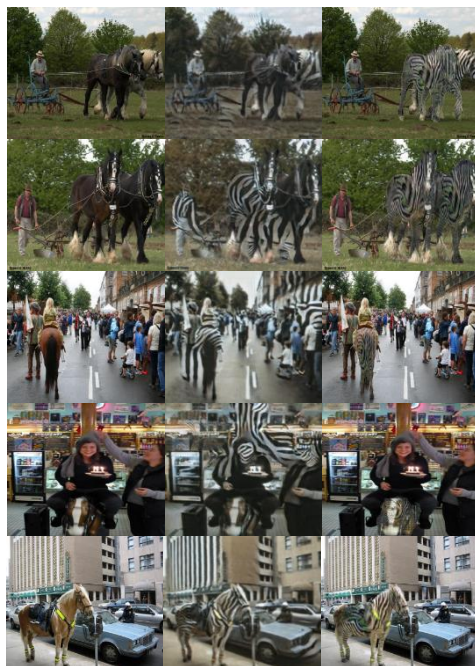

Zebra -&gt; Horse

Input

CycleGAN

Ours

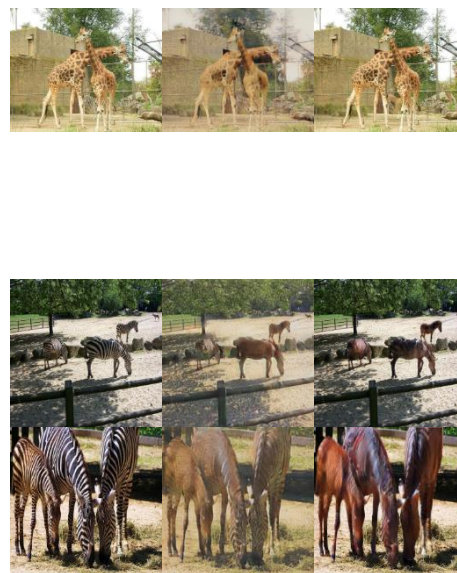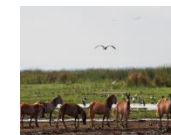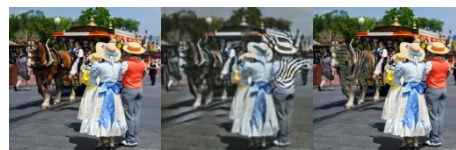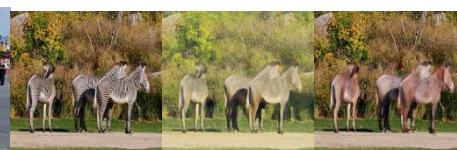

Supplement: Supplementary file 1 [file supple.pdf]
