# Supplementary material for: Generative Semantic Manipulation with Contrasting GAN
Source: arXiv:1708.00315 source file (2017-08-01)

Input

Mask  
CycleGANMask  
contrast-GAN

Input

Mask  
CycleGANMask  
contrast-GAN

Dog -&gt; Cat

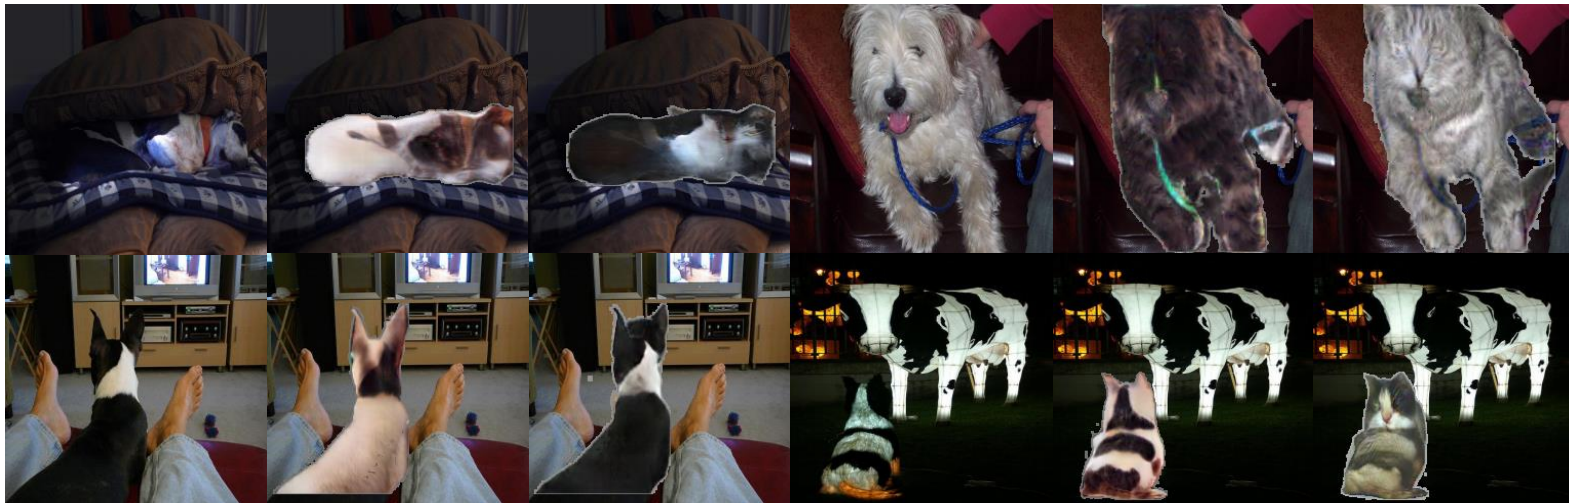

Cat -&gt; Dog

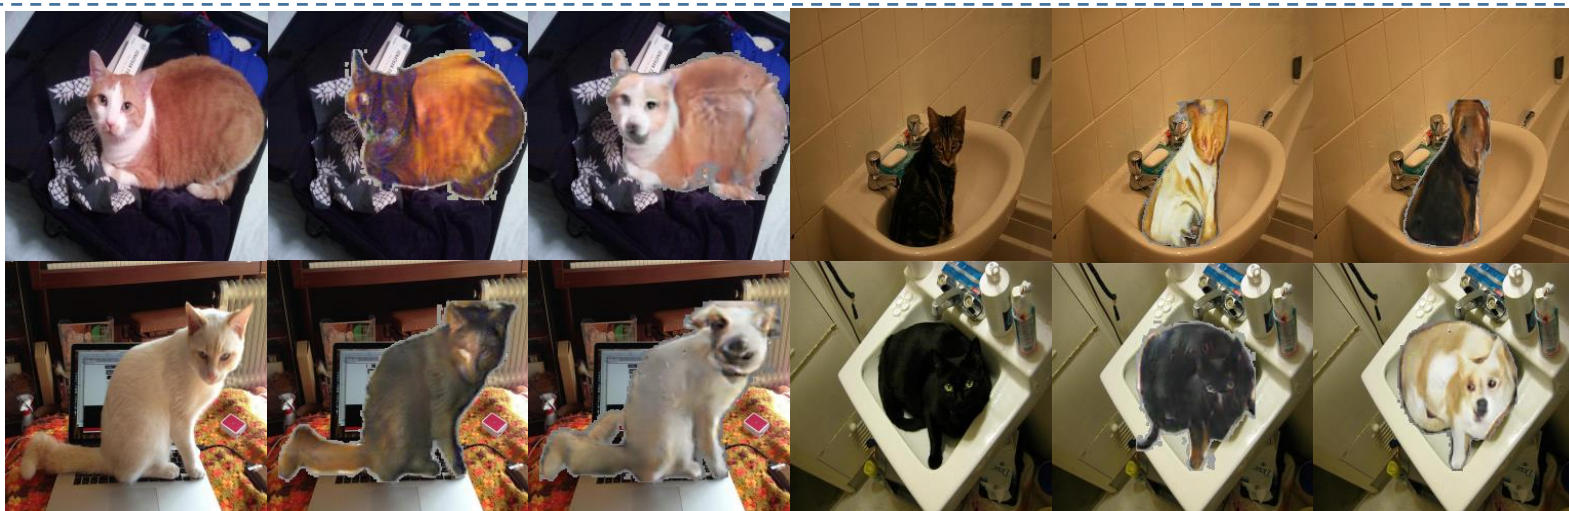

Horse -&gt; Zebra

Input

CycleGAN

Ours

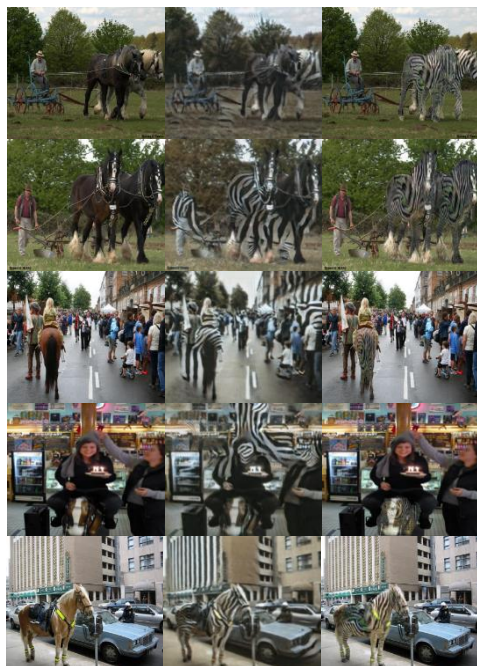

Zebra -&gt; Horse

Input

CycleGAN

Ours

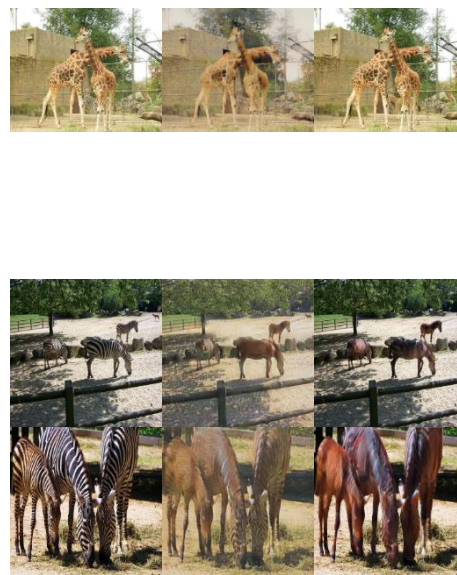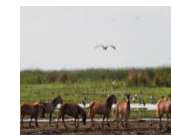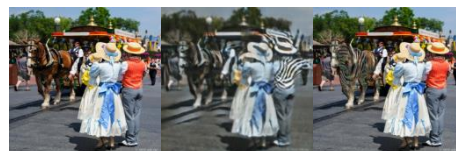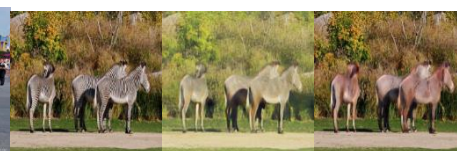

Supplement: Supplementary file 2 [file supple_mask.pdf]
