# Supplementary material for: Generative Semantic Manipulation with Contrasting GAN
Source: arXiv:1708.00315 source file (2017-08-01)

Motorcycle

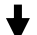

Bicycle

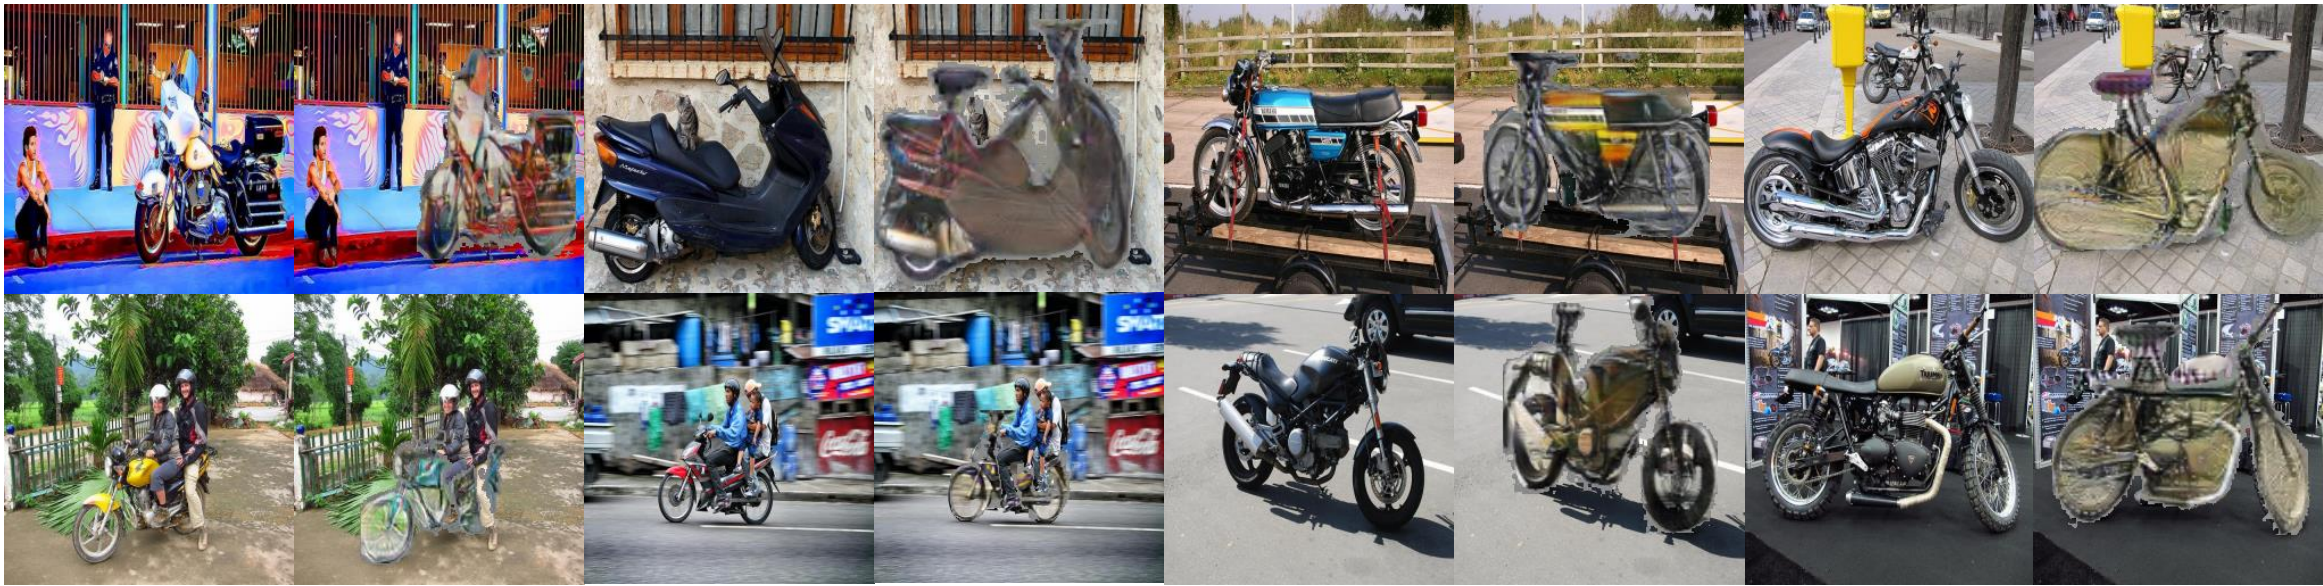

Bicycle

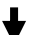

Motorcycle

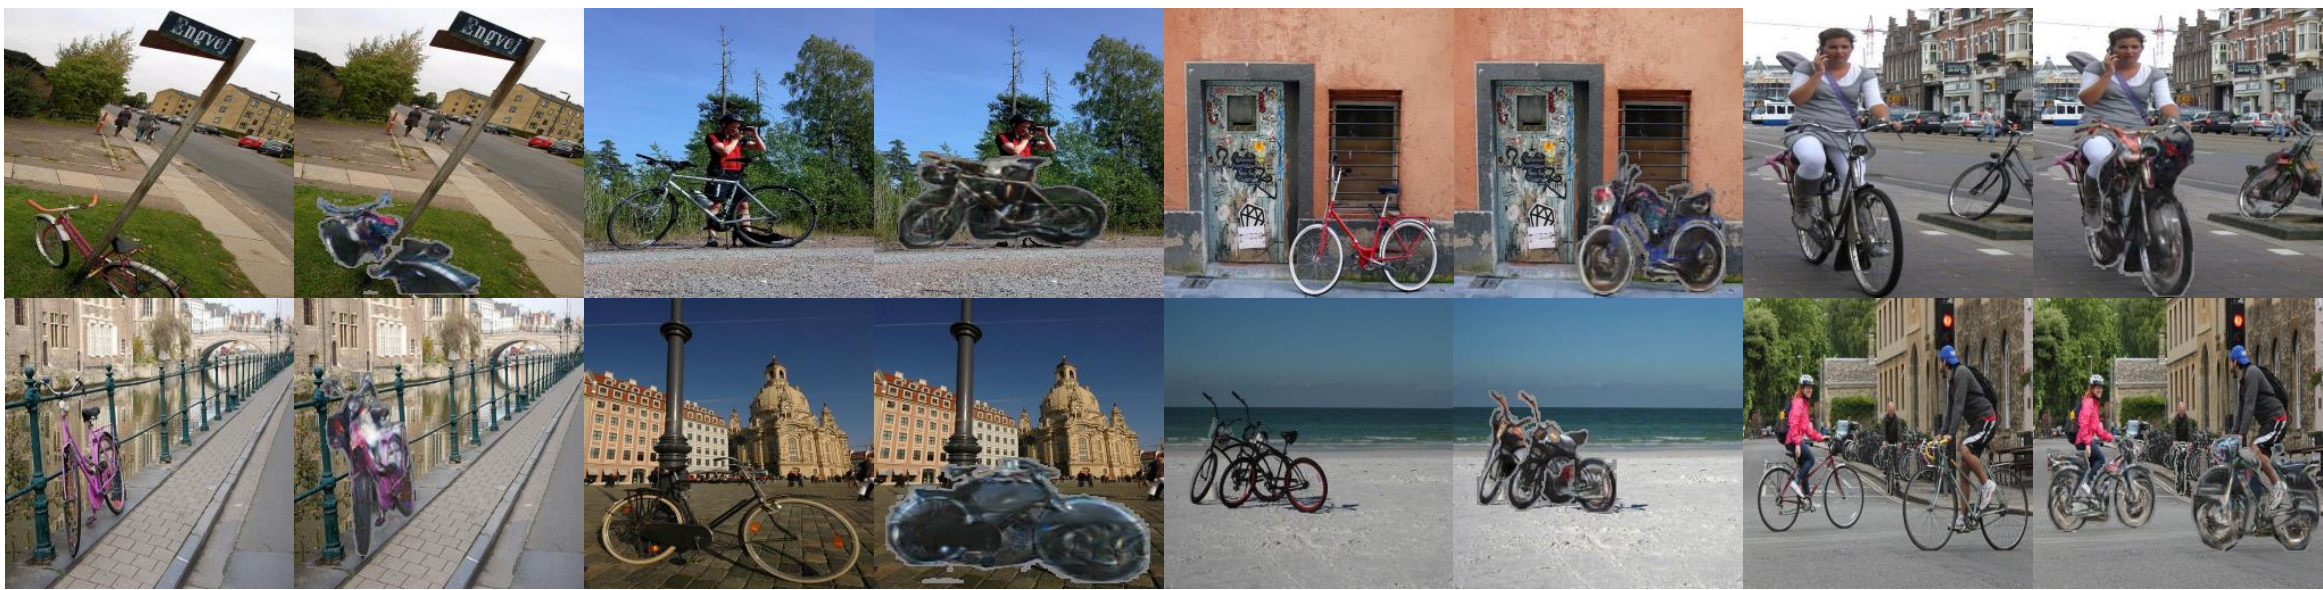



Horse -> Zebra

Input

CycleGAN

Ours

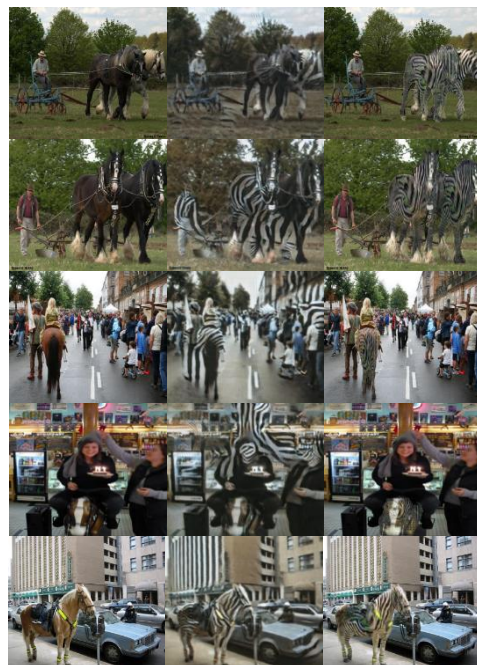

Zebra -> Horse

Input

CycleGAN

Ours

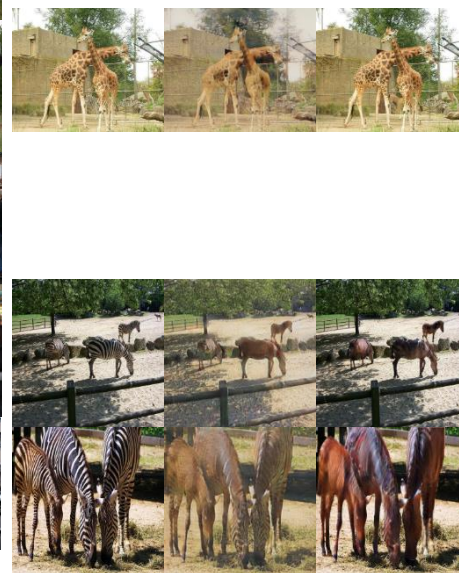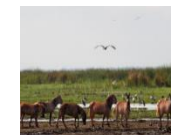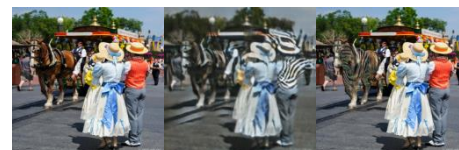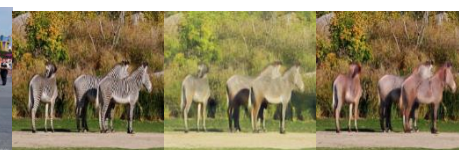

Supplement: Supplementary file 3 [file supple_results.pdf]
