# Supplementary material for: Generative Semantic Manipulation with Contrasting GAN
Source: arXiv:1708.00315 source file (2017-08-01)

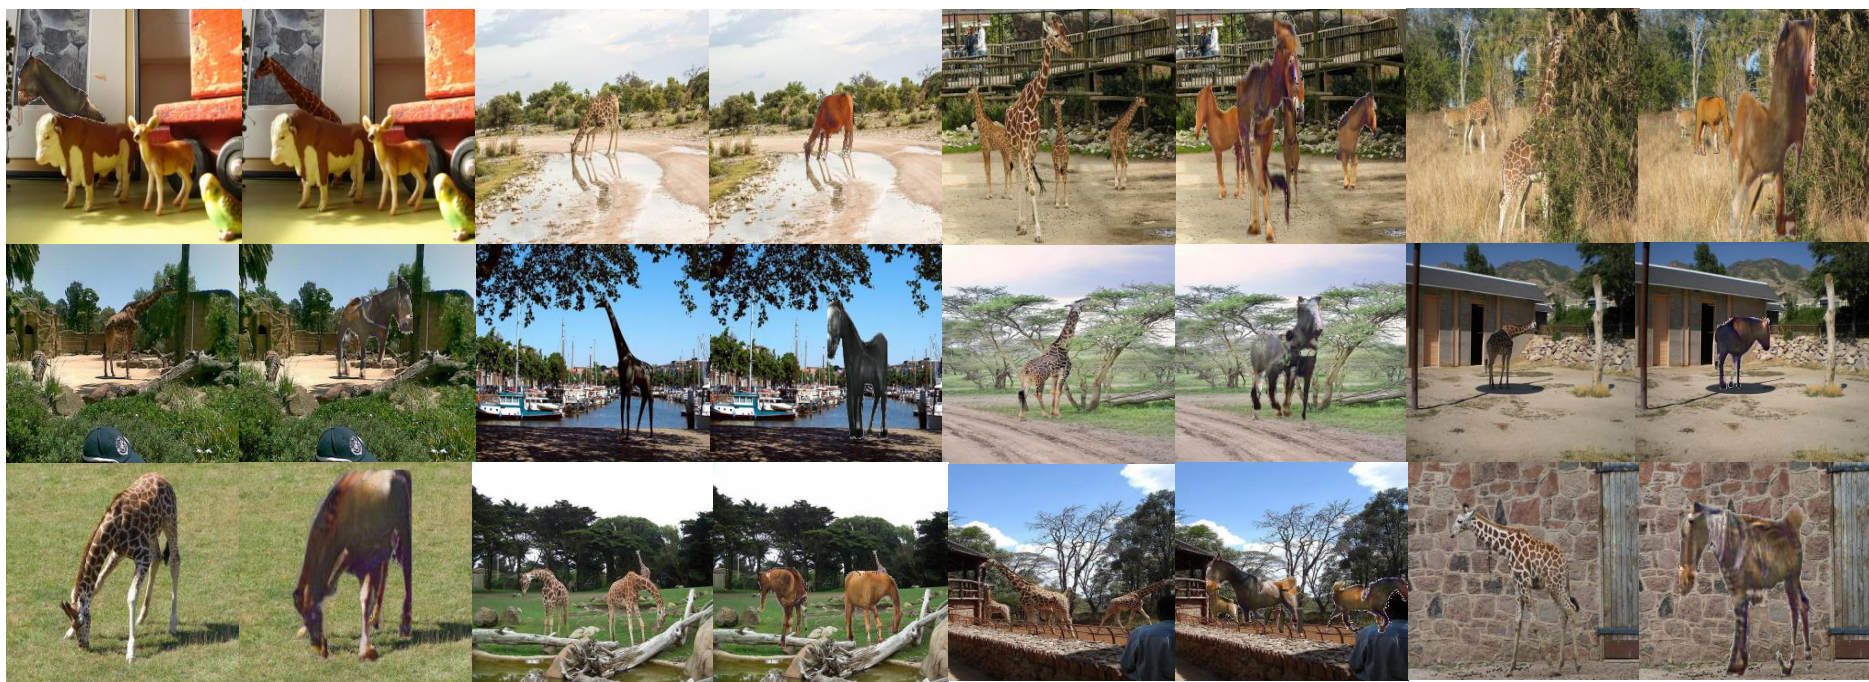

Giraffe  
↓  
Horse

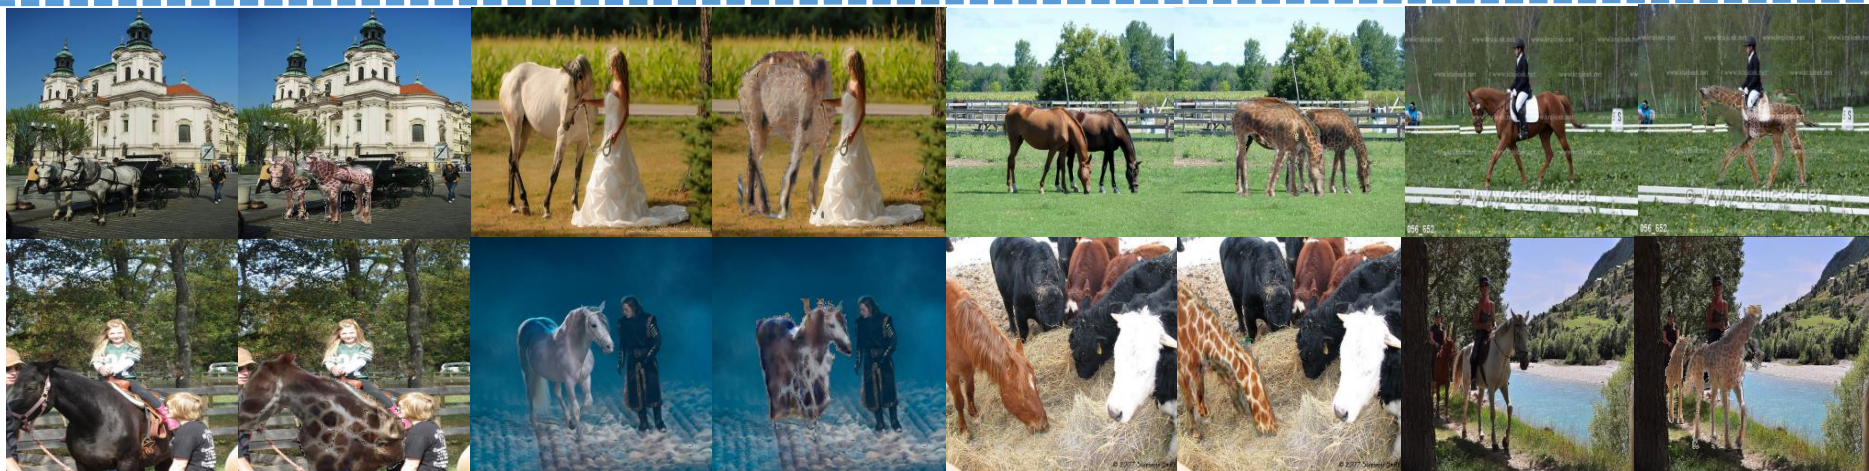

Horse  
↓  
Giraffe



Horse -&gt; Zebra

Input

CycleGAN

Ours

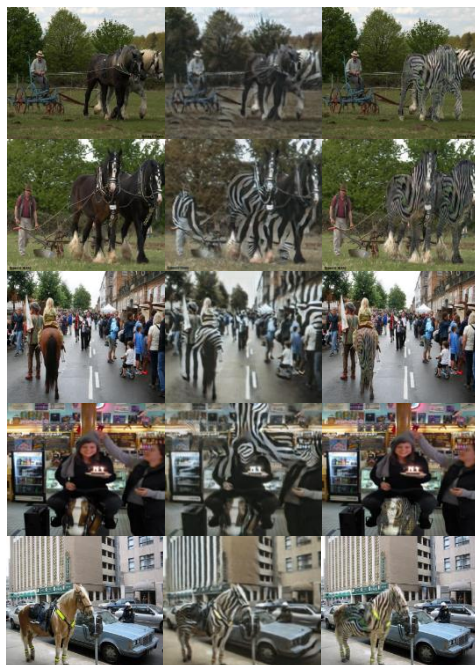

Zebra -&gt; Horse

Input

CycleGAN

Ours

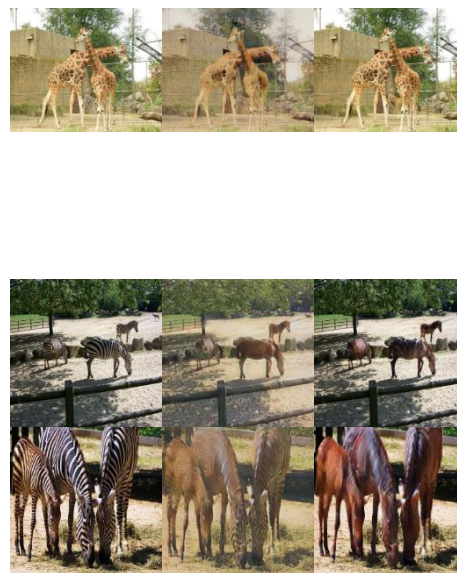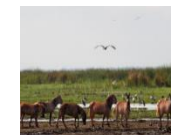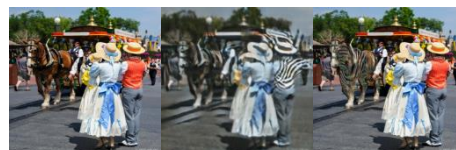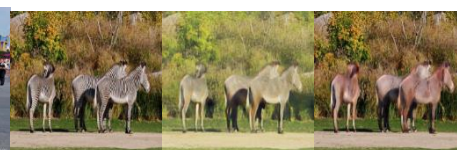

Supplement: Supplementary file 4 [file supple_results2.pdf]
